# Supplementary material for: Multigrid p-Robustness at Jacobi Speeds: Efficient Matrix-Free Implementation of Local p-Multigrid Solvers
Source: arXiv:2512.02577 source file (2025-12-02)
Supplement: Supplementary file 1 [file appendix.tex]

\section{Dynamic Patch Distribution Algorithm}

The `Dynamic` distributor maps degrees of freedom (DoFs) between local cell storage and global patch storage without
precomputed tables. The mapping is computed on the fly via a recursive tensor-product traversal. The algorithm relies
on three user-provided functors:
\begin{itemize}
    \item $\Phi_{reg}(\mathcal{I}_{patch}, c, \mathcal{I}_{cell})$: Processes a DoF owned by the current cell.
    \item $\Phi_{dup}(\mathcal{I}_{patch}, c, \mathcal{I}_{cell})$: Processes a DoF shared with a neighbor (overlap/ghost).
    \item $\Phi_{skip}(c, \mathcal{I}_{cell})$: Processes a DoF that is not part of the patch vector (e.g., external boundaries).
\end{itemize}

Those functors encapsulate the actual data movement, allowing the traversal algorithm to remain agnostic of the
specific data operations.

\subsection{The 1D Base Case}
The base case processes a line of $p+1$ DoFs -- Algorithm~\ref{alg:dynamic_1D}. It accepts the current cell index $c$,
the functors, a state flag $S$, and references to the running counters for the local cell index ($\mathcal{I}_{cell}$)
and global patch index ($\mathcal{I}_{patch}$). It call functions that process left and right cells separately
(Algorithms ~\ref{alg:dynamic_1d_left} and ~\ref{alg:dynamic_1d_right}). Depending on the position along the line, they
invoke the appropriate functor. The state flag $S$ indicates whether all the DoFs in the current cell are to be skipped
(e.g., due to boundary conditions). In such cases, the algorithm bypasses the regular and overlapping functors,
invoking only the skip functor for each DoF.

\begin{algorithm}
    \caption{Wrapper for 1D Dynamic Traversal}
    \label{alg:dynamic_1D}
    \begin{algorithmic}[1]
        \Function{Traverse1D}{$c$, $\dots$}
        \If{$c$ is Left ($0$)}
        \State \Call{Traverse1D\_Left}{$\dots$}
        \Else
        \State \Call{Traverse1D\_Right}{$\dots$}
        \EndIf
        \State \Return
        \EndFunction
    \end{algorithmic}
\end{algorithm}

\begin{algorithm}
    \caption{1D Dynamic Traversal: Left Cell ($c=0$)}
    \label{alg:dynamic_1d_left}
    \begin{algorithmic}[1]
        \Function{Traverse1D\_Left}{$\Phi_{reg}, \Phi_{skip}, S, \mathcal{I}_{cell}, \mathcal{I}_{patch}$}
        \State Let $K$ be the patch stride (1 in 1D).

        \State $\Phi_{skip}(c, \mathcal{I}_{cell})$ \Comment{\textbf{Node 0}: Outer Boundary (Always Skipped)}
        \State $\mathcal{I}_{cell} \mathrel{+}= 1$

        \For{$k = 1 \dots p-1$} \Comment{\textbf{Nodes $1 \dots p-1$}: Interior}
        \If{$S$}
        \State $\Phi_{skip}(c, \mathcal{I}_{cell})$
        \Else
        \State $\Phi_{reg}(\mathcal{I}_{patch}, c, \mathcal{I}_{cell})$
        \State $\mathcal{I}_{patch} \mathrel{+}= K$
        \EndIf
        \State $\mathcal{I}_{cell} \mathrel{+}= 1$
        \EndFor

        \If{$S$}  \Comment{\textbf{Node $p$}: Shared Interface (Owner)}
        \State $\Phi_{skip}(c, \mathcal{I}_{cell})$
        \Else
        \State $\Phi_{reg}(\mathcal{I}_{patch}, c, \mathcal{I}_{cell})$
        \State $\mathcal{I}_{patch} \mathrel{+}= K$
        \EndIf
        \State $\mathcal{I}_{cell} \mathrel{+}= 1$
        \EndFunction
    \end{algorithmic}
\end{algorithm}

\begin{algorithm}
    \caption{1D Dynamic Traversal: Right Cell ($c=1$)}
    \label{alg:dynamic_1d_right}
    \begin{algorithmic}[1]
        \Function{Traverse1D\_Right}{$ \Phi_{reg}, \Phi_{dup}, \Phi_{skip}, S, \mathcal{I}_{cell}, \mathcal{I}_{patch}$}
        \State Let $K$ be the patch stride (1 in 1D).

        \If{$S$} \Comment{\textbf{Node 0}: Shared Interface (Overlap)}
        \State $\Phi_{skip}(c, \mathcal{I}_{cell})$
        \Else
        \State $\Phi_{dup}(\mathcal{I}_{patch}, c, \mathcal{I}_{cell})$
        \State $\mathcal{I}_{patch} \mathrel{+}= K$
        \EndIf
        \State $\mathcal{I}_{cell} \mathrel{+}= 1$

        \For{$k = 1 \dots p-1$} \Comment{\textbf{Nodes $1 \dots p-1$}: Interior}
        \If{$S$}
        \State $\Phi_{skip}(c, \mathcal{I}_{cell})$
        \Else
        \State $\Phi_{reg}(\mathcal{I}_{patch}, c, \mathcal{I}_{cell})$
        \State $\mathcal{I}_{patch} \mathrel{+}= K$
        \EndIf
        \State $\mathcal{I}_{cell} \mathrel{+}= 1$
        \EndFor

        \State $\Phi_{skip}(c, \mathcal{I}_{cell})$ \Comment{\textbf{Node $p$}: Outer Boundary (Always Skipped)}
        \State $\mathcal{I}_{cell} \mathrel{+}= 1$
        \EndFunction
    \end{algorithmic}
\end{algorithm}

\subsection{Recursive Generalization}
For dimension $d > 1$, the function decomposes the element into $(d-1)$-dimensional slices. The topology of the patch
is handled by permuting the functors passed to the recursive calls. Specifically, when processing a face that
represents an overlap with a previously visited neighbor, the recursion replaces $\Phi_{reg}$ with $\Phi_{dup}$.

We define $K$ as the \textit{patch stride} associated with the current dimension of recursion $d$. It represents the
memory offset required to advance from the start of one $(d-1)$-dimensional slice to the next within the flattened
global patch vector. Since the vertex patch is constructed from the union of $2^d$ cells of polynomial degree $p$, the
global number of degrees of freedom along any single coordinate axis is $N_{\text{1D}} = 2p - 1$ (accounting for the
shared central vertex). Consequently, the stride $K$ is given by the size of the tensor slice orthogonal to the
dimension being traversed:
\begin{itemize}
    \item For $d=2$ (stepping between 1D lines), the stride is the global line width:
          \[ K = 2p - 1 \]
    \item For $d=3$ (stepping between 2D planes), the stride is the global plane area:
          \[ K = (2p - 1)^2 \]
\end{itemize}
These values are compile-time constants, allowing the algorithm to navigate the global tensor structure efficiently using simple integer arithmetic.

The entire traversal logic is implemented as a C++ template parameterized by the polynomial degree $p$. This design
choice ensures that loop bounds and stride constants $K$ are known at compile time. Consequently, modern compilers can
fully inline the recursive calls and unroll the internal loops, reducing the runtime overhead of the traversal to a
sequence of direct memory accesses. Furthermore, the traversal order is designed to access degrees of freedom within
the local cell vector ($\mathcal{I}_{cell}$) consecutively, maximizing spatial locality and allowing for efficient
vectorization of the underlying data movement operations.

\begin{algorithm}
    \caption{Recursive Dynamic Traversal}
    \begin{algorithmic}[1]
        \Function{Traverse}{$d$, $c$, $\Phi_{reg}, \Phi_{dup}, \Phi_{skip}$, $S$, $\mathcal{I}_{cell}$, $\mathcal{I}_{patch}$}
        \If{$d=1$}
        \State \Call{Traverse1D}{$c$, $\Phi_{reg}, \Phi_{dup}, \Phi_{skip}$, $S$, $\mathcal{I}_{cell}$, $\mathcal{I}_{patch}$}
        \State \Return
        \EndIf

        \State Let $K$ be the patch stride for dimension $d$.
        \State Let $b_d$ be the bit of $c$ for dimension $d$ ($0=$ Left/Bottom, $1=$ Right/Top).

        \If{$b_d = 0$}
        \State \Call{Traverse}{$d-1$, $c$, $\Phi_{reg}, \Phi_{dup}, \Phi_{skip}$, \textbf{true}, $\mathcal{I}_{cell}$, $\mathcal{I}_{patch}$} \Comment{\textbf{Bottom Face}: Outer Boundary}

        \For{$k = 1 \dots p-1$}
        \State \Call{Traverse}{$d-1$, $c$, $\Phi_{reg}, \Phi_{dup}, \Phi_{skip}$, $S$, $\mathcal{I}_{cell}$, $\mathcal{I}_{patch}$}
        \Comment{\textbf{Interior Slices}}
        \If{\textbf{not} $S$} $\mathcal{I}_{patch} \mathrel{+}= K$ \EndIf
        \EndFor

        \State \Call{Traverse}{$d-1$, $c$, $\Phi_{reg}, \Phi_{dup}, \Phi_{skip}$, $S$, $\mathcal{I}_{cell}$, $\mathcal{I}_{patch}$}  \Comment{\textbf{Top Face}: Shared Interface (Owner)}
        \If{\textbf{not} $S$} $\mathcal{I}_{patch} \mathrel{+}= K$ \EndIf

        \Else \quad ($b_d = 1$)
        \State \textit{// Pass $\Phi_{dup}$ as the regular operator for the sub-face}
        \State \Call{Traverse}{$d-1$, $c$, $\boldsymbol{\Phi_{dup}}, \Phi_{dup}, \Phi_{skip}$, $S$, $\mathcal{I}_{cell}$, $\mathcal{I}_{patch}$}
        \Comment{\textbf{Bottom Face}: Shared Interface (Overlap)}
        \If{\textbf{not} $S$} $\mathcal{I}_{patch} \mathrel{+}= K$ \EndIf

        \For{$k = 1 \dots p-1$} \Comment{\textbf{Interior Slices}}
        \State \Call{Traverse}{$d-1$, $c$, $\Phi_{reg}, \Phi_{dup}, \Phi_{skip}$, $S$, $\mathcal{I}_{cell}$, $\mathcal{I}_{patch}$}
        \If{\textbf{not} $S$} $\mathcal{I}_{patch} \mathrel{+}= K$ \EndIf
        \EndFor

        \State \Call{Traverse}{$d-1$, $c$, $\Phi_{reg}, \Phi_{dup}, \Phi_{skip}$, \textbf{true}, $\mathcal{I}_{cell}$, $\mathcal{I}_{patch}$}  \Comment{\textbf{Top Face}: Outer Boundary}
        \EndIf
        \EndFunction
    \end{algorithmic}
\end{algorithm}
%%==========================================================%%
%%==========================================================%%

\section{The Lookup Patch Distributor}

In contrast to the recursive calculation of the \textit{Dynamic} approach, the \textit{Lookup} distributor relies on
precomputed static tables to map local cell degrees of freedom to the patch vector. This strategy trades program binary
size (and potential instruction cache pressure) for reduced arithmetic intensity during the smoothing operation.

The mapping information is encapsulated in a structure, specialized for each dimension $d$ and polynomial degree $p$.
These structures contain static \texttt{constexpr} arrays that store the mapping data, allowing the compiler to embed
the lookup tables directly into the binary. This avoids runtime initialization and dynamic memory allocation. For a
given cell $c$ in the patch, the lookup table $\mathcal{L}_c$ consists of a list of index pairs $(i_{\text{local}},
    i_{\text{patch}})$.

\subsection{Partitioned Execution Loop}

The \textit{Lookup} distributor partitions $\mathcal{L}_c$ based on the ownership status of the degrees of freedom. For
every cell $c$, the mapping indices are sorted such that DoFs unique to the cell (within the traversal order) appear
first, followed by DoFs shared with previously visited cells. This partitioning allows the distribution loop to avoid
branching logic inside the innermost iteration. The process is split into two distinct loops over the cells to separate
active data movement from skipped operations:

\begin{enumerate}
    \item \textbf{Active DoFs Loop:}
          This loop iterates over all cells $c$ to process degrees of freedom that participate in the patch operation. For each cell, it executes two consecutive phases:
          \begin{itemize}
              \item \textbf{Non-Overlapping (Regular) Phase:}
                    Iterates from $k = 0$ to $N_{\text{unique}}^{(c)} - 1$.
                    The operation $\Phi_{reg}$ is applied to the pair $\mathcal{L}_c[k]$. These DoFs are encountered for the first time in the current patch traversal.
              \item \textbf{Overlapping Phase:}
                    Iterates from $k = N_{\text{unique}}^{(c)}$ to $N_{\text{total}}^{(c)} - 1$.
                    The operation $\Phi_{dup}$ is applied. These DoFs correspond to interfaces shared with already-processed neighbors. In an assembly context, this typically implies accumulation rather than assignment.
          \end{itemize}

    \item \textbf{Skipped Phase:}
          After the active DoFs have been processed for all cells, a second loop iterates over the cells to handle skipped DoFs.
          A separate list $\mathcal{S}_c$ contains local DoF indices that are not part of the patch vector (e.g., boundary nodes). The operation $\Phi_{skip}$ is applied to these indices.
\end{enumerate}

This structure is formalized in Algorithm~\ref{alg:lookup_distributor}.

\begin{algorithm}[t]
    \caption{Table-Driven Lookup Traversal}
    \label{alg:lookup_distributor}
    \begin{algorithmic}[1]
        \Require Precomputed tables $\mathcal{L}$, cutoffs $N_{\text{unique}}$, $N_{\text{total}}$, skipped lists $\mathcal{S}$
        \For{$c \gets 0 \textbf{ to } N_{\text{cells}} - 1$}
        \Comment{Phase 1: Unique DoFs}
        \For{$k \gets 0 \textbf{ to } N_{\text{unique}}^{(c)} - 1$}
        \State $(u, v) \gets \mathcal{L}_c[k]$
        \State $\Phi_{reg}(v, c, u)$ \Comment{Global index $v$, Cell $c$, Local index $u$}
        \EndFor

        \For{$k \gets N_{\text{unique}}^{(c)} \textbf{ to } N_{\text{total}}^{(c)} - 1$}
        \Comment{Phase 2: Shared DoFs}
        \State $(u, v) \gets \mathcal{L}_c[k]$
        \State $\Phi_{dup}(v, c, u)$
        \EndFor
        \EndFor

        \For{$c \gets 0 \textbf{ to } N_{\text{cells}} - 1$}
        \For{$u \textbf{ in } \mathcal{S}_c$}
        \Comment{Phase 3: Skipped DoFs}
        \State $\Phi_{skip}(c, u)$
        \EndFor
        \EndFor
    \end{algorithmic}
\end{algorithm}
